# Supplementary material for: SpheriColor: Colormaps for Spherical Geospatial Input Topographies
Source: arXiv:2610.11470 source file (2026-10-08)
Supplement: Supplementary file 3 [file _appendix_eurovis.tex]

% ---------------------------------------------------------------------------
% Author guideline and sample document for EG publication using LaTeX2e input
% D.Fellner, v1.21, Jan 08, 2024

\documentclass{egpubl}
\usepackage{eurovis2026}

\ShortPresentation      % uncomment for (final) Short Conference  
\EuroVisShort  % for EuroVis additional material
%                          % EuroVis, SGP, Rendering, PG
%\CGFStandardLicense
\CGFccby
%\CGFccbync
%\CGFccbyncnd

\usepackage[T1]{fontenc}
\usepackage{dfadobe}  

\usepackage{subcaption}
\usepackage{tabularx}

\usepackage{cite}  % comment out for biblatex with backend=biber
\BibtexOrBiblatex
\electronicVersion
\PrintedOrElectronic
\ifpdf \usepackage[pdftex]{graphicx} \pdfcompresslevel=9
\else \usepackage[dvips]{graphicx} \fi

\usepackage{egweblnk}
% end of prologue

\input{sections/_preamble}

\title[\papertitle~-- Supplementary Material]%
      {\papertitle \\ Supplementary Material}

\author[SUBMISSION ID 1054]{SUBMISSION ID 1054}


\begin{document}
\maketitle


%\appendix
% change figure appendix style
\renewcommand{\thefigure}{A.\arabic{figure}}
\setcounter{figure}{0}




%\vspace{2\baselineskip}

\input{sections/_appendix_content}

% bibtex
%\bibliographystyle{eg-alpha-doi} 
%\bibliography{references/refs}       

\end{document}
