# Supplementary material for: SpheriColor: Colormaps for Spherical Geospatial Input Topographies
Source: arXiv:2610.11470 source file (2026-10-08)
Supplement: Supplementary file 4 [file _appendix_vis.tex]

% $Id: template.tex 11 2007-04-03 22:25:53Z jpeltier $

\documentclass{vgtc}                          % final (conference style)
%\documentclass[review]{vgtc}                 % review


%% it is recomended to use ``\cref{sec:bla}'' instead of ``Fig.~\ref{sphericolor:sec:bla}''
\graphicspath{{content/papers/sphericolor/figures/}{pictures/}{images/}{./}} % where to search for the images

\usepackage{times}                     % we use Times as the main font
\renewcommand*\ttdefault{txtt}         % a nicer typewriter font

%% Only used in the template examples. You can remove these lines.
\usepackage{tabu}                      % only used for the table example
\usepackage{booktabs}                  % only used for the table example
\usepackage{lipsum}                    % used to generate placeholder text
\usepackage{mwe}                       % used to generate placeholder figures

%% We encourage the use of mathptmx for consistent usage of times font
%% throughout the proceedings. However, if you encounter conflicts
%% with other math-related packages, you may want to disable it.
\usepackage{mathptmx}                  % use matching math font


%% If you are submitting a paper to a conference for review with a double
%% blind reviewing process, please replace the value ``0'' below with your
%% OnlineID. Otherwise, you may safely leave it at ``0''.
\onlineid{1182}

%% declare the category of your paper, only shown in review mode
\vgtccategory{Research}

%% allow for this line if you want the electronic option to work properly
\vgtcinsertpkg

%% In preprint mode you may define your own headline. If not, the default IEEE copyright message will appear in preprint mode.
%\preprinttext{To appear in an IEEE VGTC sponsored conference.}

%% This adds a link to the version of the paper on IEEEXplore
%% Uncomment this line when you produce a preprint version of the article 
%% after the article receives a DOI for the paper from IEEE
%\ieeedoi{xx.xxxx/TVCG.201x.xxxxxxx}


%% Paper title.

\input{sections/_preamble}

\title{\papertitle \\ Supplementary Material}

%% This is how authors are specified in the conference style

%% Author and Affiliation (single author).
%%\author{Roy G. Biv\thanks{e-mail: roy.g.biv@aol.com}}
%%\affiliation{\scriptsize Allied Widgets Research}

%% Author and Affiliation (multiple authors with single affiliations).
%%\author{Roy G. Biv\thanks{e-mail: roy.g.biv@aol.com} %
%%\and Ed Grimley\thanks{e-mail:ed.grimley@aol.com} %
%%\and Martha Stewart\thanks{e-mail:martha.stewart@marthastewart.com}}
%%\affiliation{\scriptsize Martha Stewart Enterprises \\ Microsoft Research}

%% Author and Affiliation (multiple authors with multiple affiliations)
\author{Julius Rauscher\thanks{e-mail: {firstname.lastname}@uni-konstanz.de}\\ %
        \scriptsize University of Konstanz %
\and Johannes Fuchs\\ %
     \scriptsize University of Konstanz %
 \and Daniel A. Keim\\ %
     \scriptsize University of Konstanz %
      \and Frederik L. Dennig\\ %
     \scriptsize University of Konstanz }



%% Copyright space is enabled by default as required by guidelines.
%% It is disabled by the 'review' option or via the following command:
% \nocopyrightspace

%%%%%%%%%%%%%%%%%%%%%%%%%%%%%%%%%%%%%%%%%%%%%%%%%%%%%%%%%%%%%%%%
%%%%%%%%%%%%%%%%%%%%%% START OF THE PAPER %%%%%%%%%%%%%%%%%%%%%%
%%%%%%%%%%%%%%%%%%%%%%%%%%%%%%%%%%%%%%%%%%%%%%%%%%%%%%%%%%%%%%%%%

\begin{document}

\maketitle
 

\input{sections/_appendix_content}

\end{document}
